# Supplementary material for: A Shared Parameter Model for Systolic Blood Pressure Accounting for Data Missing Not at Random in the HUNT Study
Source: arXiv:2203.16602 source file (2022-03-30)
Supplement: Supplementary file 1 [file simulated_data.tex]

\section{Simulated Data for Reproducability Purposes}
\label{sec:reproducibility}

To follow the standard of high-end journals such as the Journal of the American Statistical Association, we have chosen to make all code publicly available and generate a simulated dataset. These can be found in the following GitHub repository: \cite{git_repo}. For reproducibility reasons, the best would be to make all data available. However, data from the HUNT study contains sensitive personal information and can not be shared. To enable third parties to evaluate the methods and findings of this work, we have constructed a simulated dataset with similar properties as the original data.

The explanatory variables are generated based on graphical inspection, summary statistics of the HUNT2 cohort including empirical correlations, and simple linear frequentist regressions. In this chapter, we use $i$ to index the actual participants of the HUNT2 cohort and $j$ to index the simulated participants. The response variables, i.e. future blood pressures and the missing process are generated based on the posterior mean estimates of the model parameters of the SPM presented in \cref{tb:summary_param_est}. The aim has been to obtain a simulated dataset with similar properties as the HUNT2 cohort, also concerning dependence in the explanatory variables. Further formal modeling and inference regarding the models for the simulated data is outside the scope of this thesis. 

\subsection{Generation of the Explanatory Variables}
The variable $Sex$ is drawn from a binomial distribution and $age$ is drawn independently from $sex$ from a truncated mixed normal distribution.
$BMI$ is drawn from a skewed normal (SN) distribution dependent on $age$ and $sex$. Further $BP_I$ is also drawn from a SN distribution depending on $sex$, $age$, and $BMI$. 

The following paragraph consists of a detailed explanation of the simulation process for each explanatory variable.

\textbf{Sex: }
$Sex$ is drawn independently for each participant $j$ from a Bernoulli distribution with parameter $p$ equal to the fraction of female participants in HUNT2 (\cref{tb:summary_HUNT2}). 
\begin{equation*}
    sex_j {\sim}  \text{Binomial} ( p = 0.5303 )
\end{equation*}

\textbf{Age: }
$Age$ is considered independent of $sex$ and draw from a mixed normal distribution. 
\begin{equation*}
    age_j \sim 0.75N(43,15^2) + 0.25N(75,7^2)
\end{equation*}
This means, for each participant, we draw a cut parameter from a Bernoulli distribution with parameter $p = 0.75$. If the cut parameter is one, we draw age from a normal distribution with mean, $ \mu = 43$, and standard deviation, $\sigma = 15$, otherwise we draw from a normal distribution with mean $75$ and standard deviation $7$.
In addition we truncate $age$ at $age_j=18$ and $age_j = 105$. More precisely for every value of $age_j <18$ we draw a new value from distribution $N(43,15^2)$ until it was greater than $18$ and for every value of $age_j>105$ we draw a new value from $N(75,7^2)$ distribution.
Afterward, we round the $age$ to one significant digit to replicate the format used in the HUNT Study before standardizing it. We draw $age_j$ on the original scale (years) before standardizing it to ensure the same number of possible ages as in the HUNT2 cohort. 

\textbf{BMI:}
$BMI$ is correlated with both $age$ and $sex$ in HUNT2. To be able to mimic this dependency we first perform a linear regression on the HUNT2 cohort as follows,
\begin{align*}
     BMI_i = \alpha_0 + \alpha_{age} age_i + \alpha_{sex} sex_i + \epsilon_i, \\
     \epsilon_i \sim N(0, \sigma^2).
\end{align*}
The result of this linear regression can be seen in \cref{tb:lin_reg_bmi}.
\begin{table}
\centering
\caption{Coefficients of the linear regression $BMI_I = \alpha_0 + \alpha_{age} age_i + \alpha_{sex} sex_i + \epsilon_i$ with 
     $\epsilon_i \sim N(0, \sigma^2)$}
\begin{tabular}{l|c|c|c}
\textbf{Variable} & \textbf{Mean} & \textbf{Std. error} & \textbf{Pr(\textgreater{}|t|)} \\ \hline
$\alpha_0$              & -0.023        & 0.005               & 1 e-5                          \\
$\alpha_{age}$            & 0.191         & 0.004               & \textless 2e-16                \\
$\alpha_{sex}$            & 0.05          & 0.008               & 1.2 e-10                      
\end{tabular}
\label{tb:lin_reg_bmi}
\end{table}
The distribution of $BMI$ in the HUNT2 cohort is skewed compared to a normal distribution. Therefor we use a skewed normal (SN) distribution with density as follows;
\begin{equation*}
    f(x) = \frac{2}{\sigma} \phi(\frac{x - \mu}{\sigma}) \Phi(\xi (\frac{x - \mu}{\sigma}),
\end{equation*}
where $\phi(.)$ denotes the standard normal density function and $\Phi$ denotes the corresponding cumulative density function.

The SN used to generate $BMI_j$ has mean $\mu= \alpha_0 + \alpha_{age} age_j \alpha_{sex} sex_j$, standard deviation $\sigma = 0.9$ and skewness parameter $\xi= 1.5$. The coeffcients $\alpha_0$, $\alpha_{age}$, and $\alpha_{sex}$ take the values presented in \cref{tb:lin_reg_bmi} from the linear regression of $BMI$ on the HUNT2 cohort.  For each simulated participant $j$ we use the corresponding simulated $age$ and $sex$. 
\begin{equation*}
    {BMI}_j \sim SN(\mu = \alpha_0 + \alpha_{age} age_j \alpha_{sex} sex_j, \sigma = 2, \xi = 1.5)
\end{equation*}

\textbf{$\textbf{BP}_\textbf{I}$: }
$BP_I$ is correlated with $age$, $sex$, and $BMI$ in the HUNT2 cohort. Therefore we perform a linear regression on the HUNT2 cohort as follows,
\begin{align*}
     {BP_I}_i = \alpha_0 +\alpha_{sex} sex_i + \alpha_{age} age_i + \alpha_{bmi} BMI_i \epsilon_i\\
     \epsilon_i \sim N(0, \sigma^2).
\end{align*}
The results of this regression can be seen in \cref{tb:lin_reg_bp_2}.
\begin{table}
\centering
\caption{Coefficients of the linear regression $BP_I = \alpha_0 +\alpha_{sex} sex_i + \alpha_{age} age_i + \alpha_{BMI} BMI_i + \epsilon_i$ with 
     $\epsilon_i \sim N(0, \sigma^2)$ on the HUNT2 cohort.}
\begin{tabular}{l|c|c|c}
\textbf{Variable} & \textbf{Estimate} & \textbf{Std. Error} & \textbf{Pr(\textgreater{}|t|)} \\ \hline
$\alpha_0$              & -0.078            & 0.004               & \textless 2e-16                \\
$\alpha_{sex}$          & 0.167             & 0.006               & \textless 2e-16                \\
$\alpha_{age}$            & 0.516             & 0.003               & \textless 2e-16                \\
$\alpha_{BMI}$            & 0.186             & 0.003               & \textless 2e-16               
\end{tabular}
\label{tb:lin_reg_bp_2}
\end{table}
Again the true distribution is more skewed leading us to use a SN distribution with mean $\mu = \alpha_0 + \alpha_{sex}sex_j + \alpha_{age}age_j + \alpha_{bmi} BMI_j -0.15$, standard deviation $0.85$, and skewness $\xi = 3$ and where $\alpha_0$, $\alpha_{sex}$, $\alpha_{age}$, and $alpha_{BMI}$ are given in \cref{tb:lin_reg_bp_2}.
\begin{align*}
    {BP_I} \sim SN(\mu = \alpha_0 + \alpha_{sex}sex_j + \alpha_{age}age_j + \alpha_{bmi} BMI_j -0.15, \sigma = 0.6, \xi = 3) 
\end{align*}

\subsection{Generating the Response Values}
The response values $BP_F$, and $m$ are constructed using the posterior mean estimates for all model parameters from the SPM given in \cref{tb:summary_param_est} fitted to the HUNT2 cohort. 

\textbf{$\textbf{BP}_\textbf{F}$ and $\textbf{m}$: }
\begin{align*}
    \epsilon_j \sim \text{normal}(0, \sigma_{epsilon}^2) \\
    {BP_F}_j = \alpha_0 +\alpha_{sex}  sex_j + \alpha_{age} age_j + \alpha_{bmi} BMI_j + \alpha_{BP_I} {BP_I}_j + \epsilon_j \\
    \text{logit}(p_j) = \beta_0 +\beta_{sex}  sex_j + f(age_j) + \beta_{bmi} BMI_j + \beta_{BP_I} {BP_I}_j + c\epsilon_j\\
    m_j \sim \text{Bernoulli}(p_j)
\end{align*}

\subsection{Comparison Between Simulated Data and the HUNT2 Cohort}
As we can see from  \cref{fig:sim_data_comp} the distribution of $age$, $BMI$, $BP_2$ and $BP_3$ are similar. The correlation matrices for both the true and simulated data are displayed in \cref{fig:corr_true} and \cref{fig:corr_sim} and also show similar properties.

\begin{figure}
     \centering
     \begin{subfigure}{1\textwidth}
         \centering
         \includegraphics[width = 0.8\textwidth, height = 0.42\textheight]{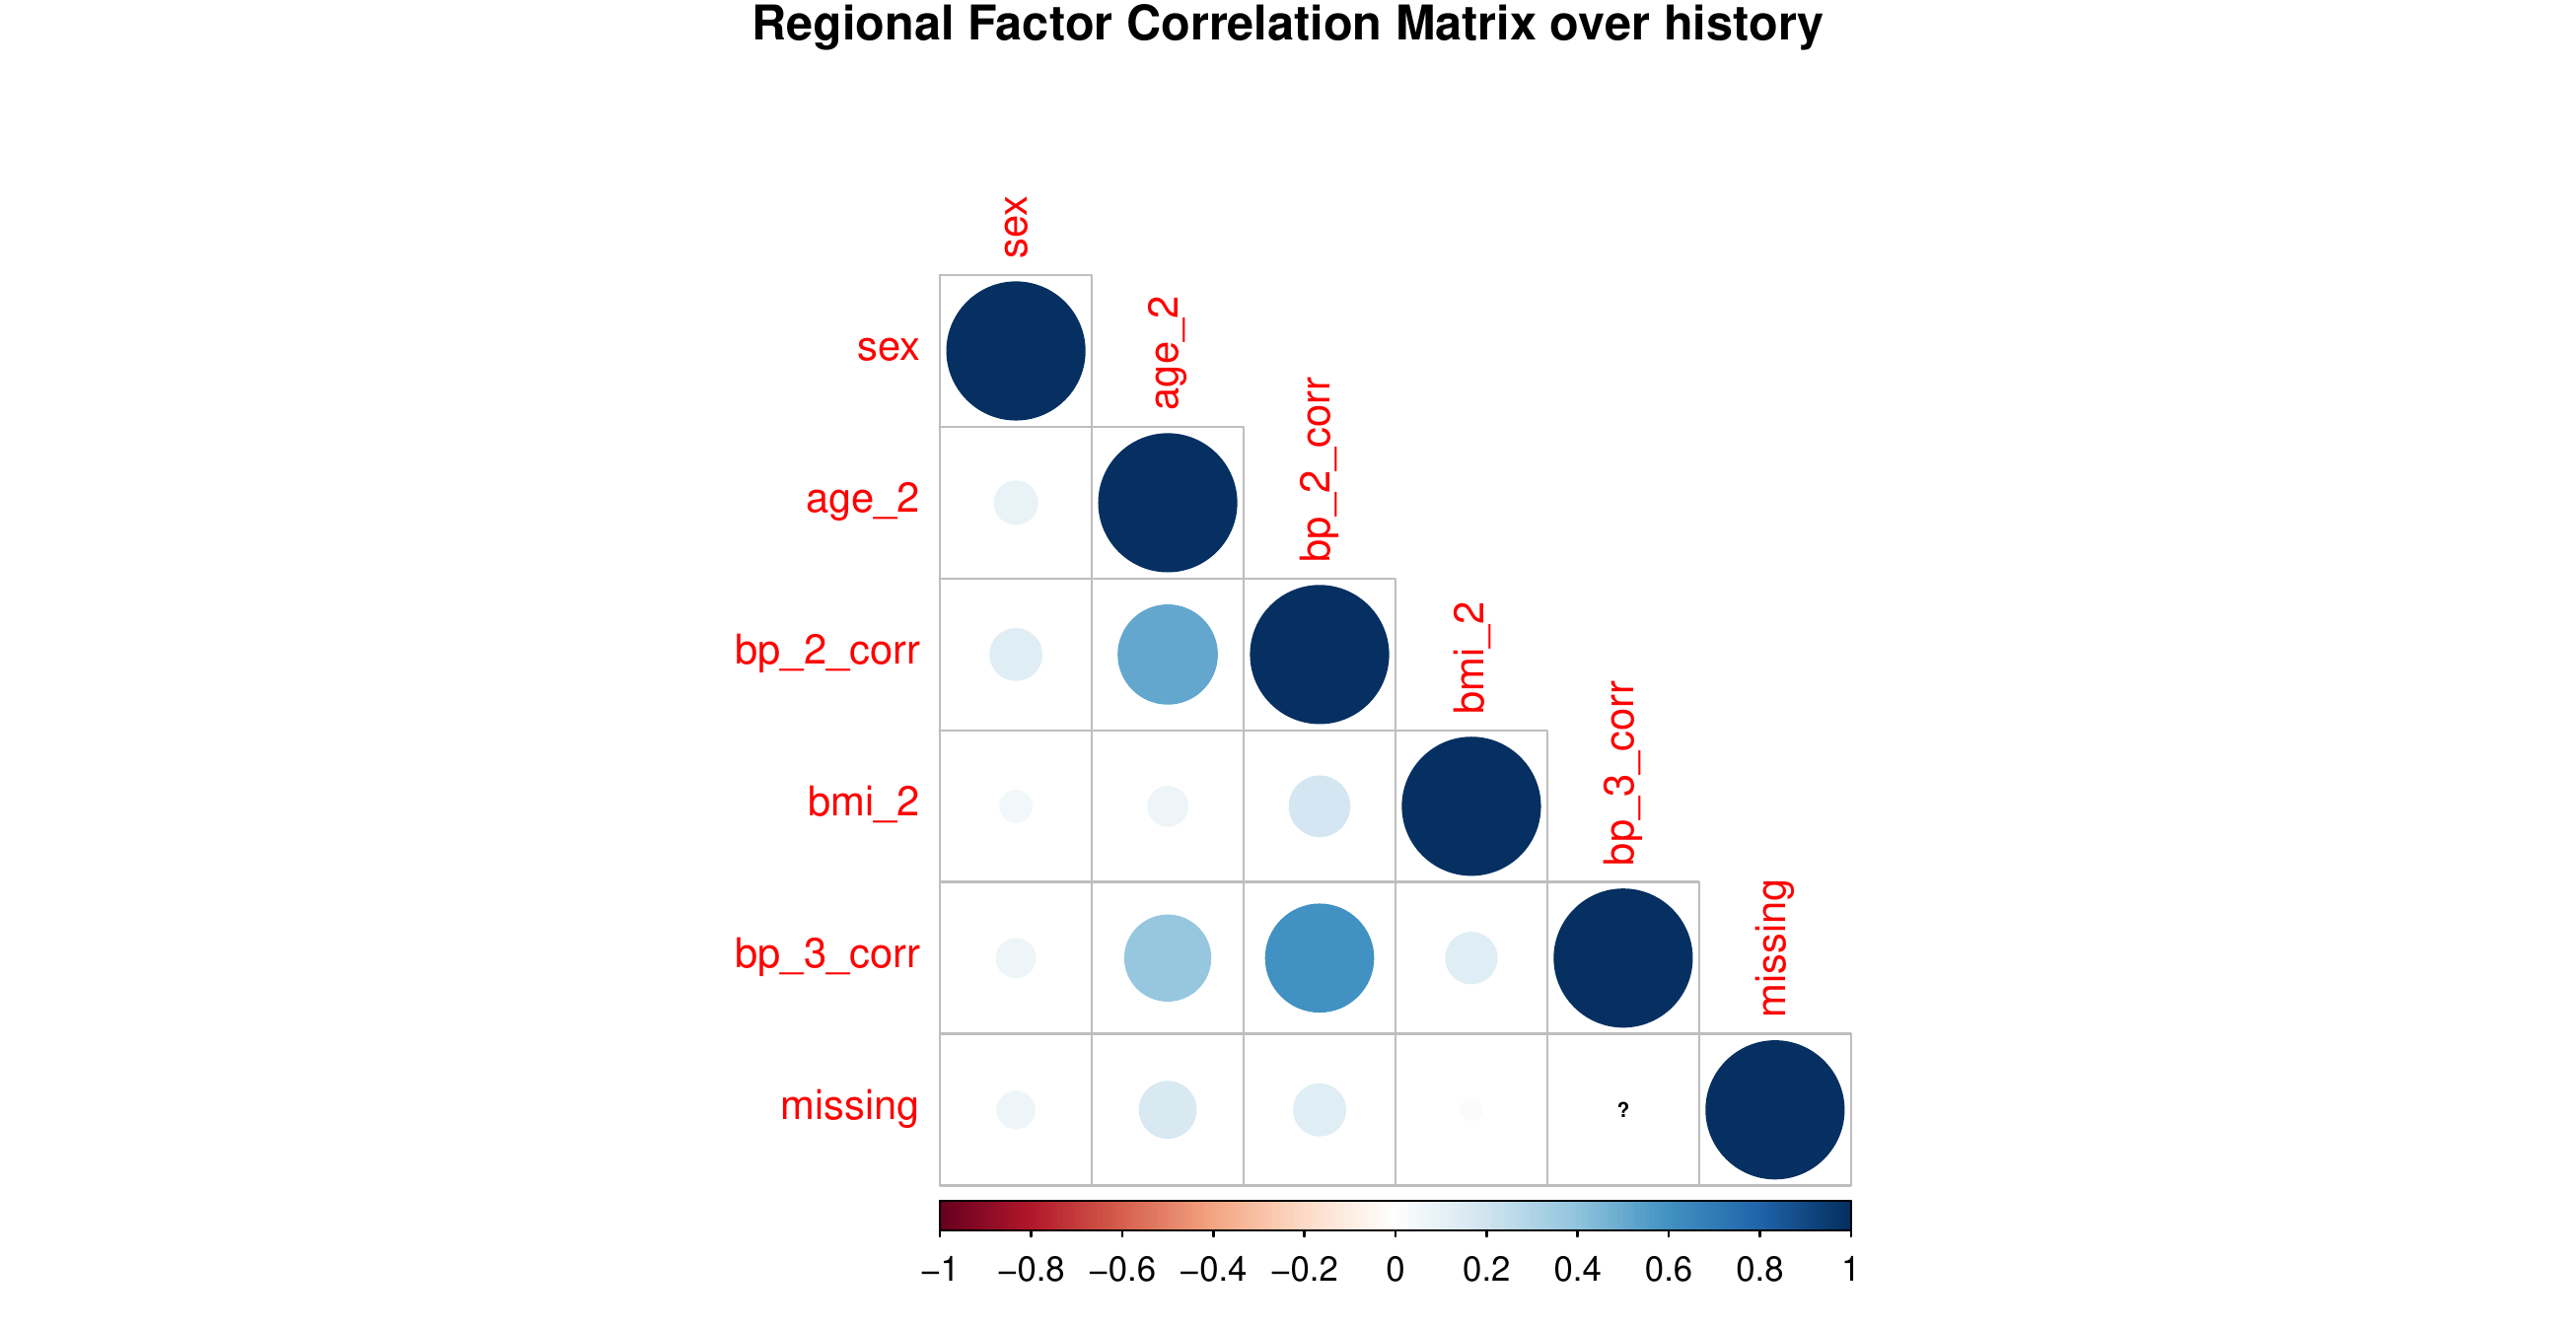}
         \caption{Correlation plot for the HUNT2 cohort.}
         \label{fig:corr_true}
     \end{subfigure}

     \begin{subfigure}{1\textwidth}
        \centering
        \includegraphics[width = 0.8\textwidth, height = 0.42\textheight]{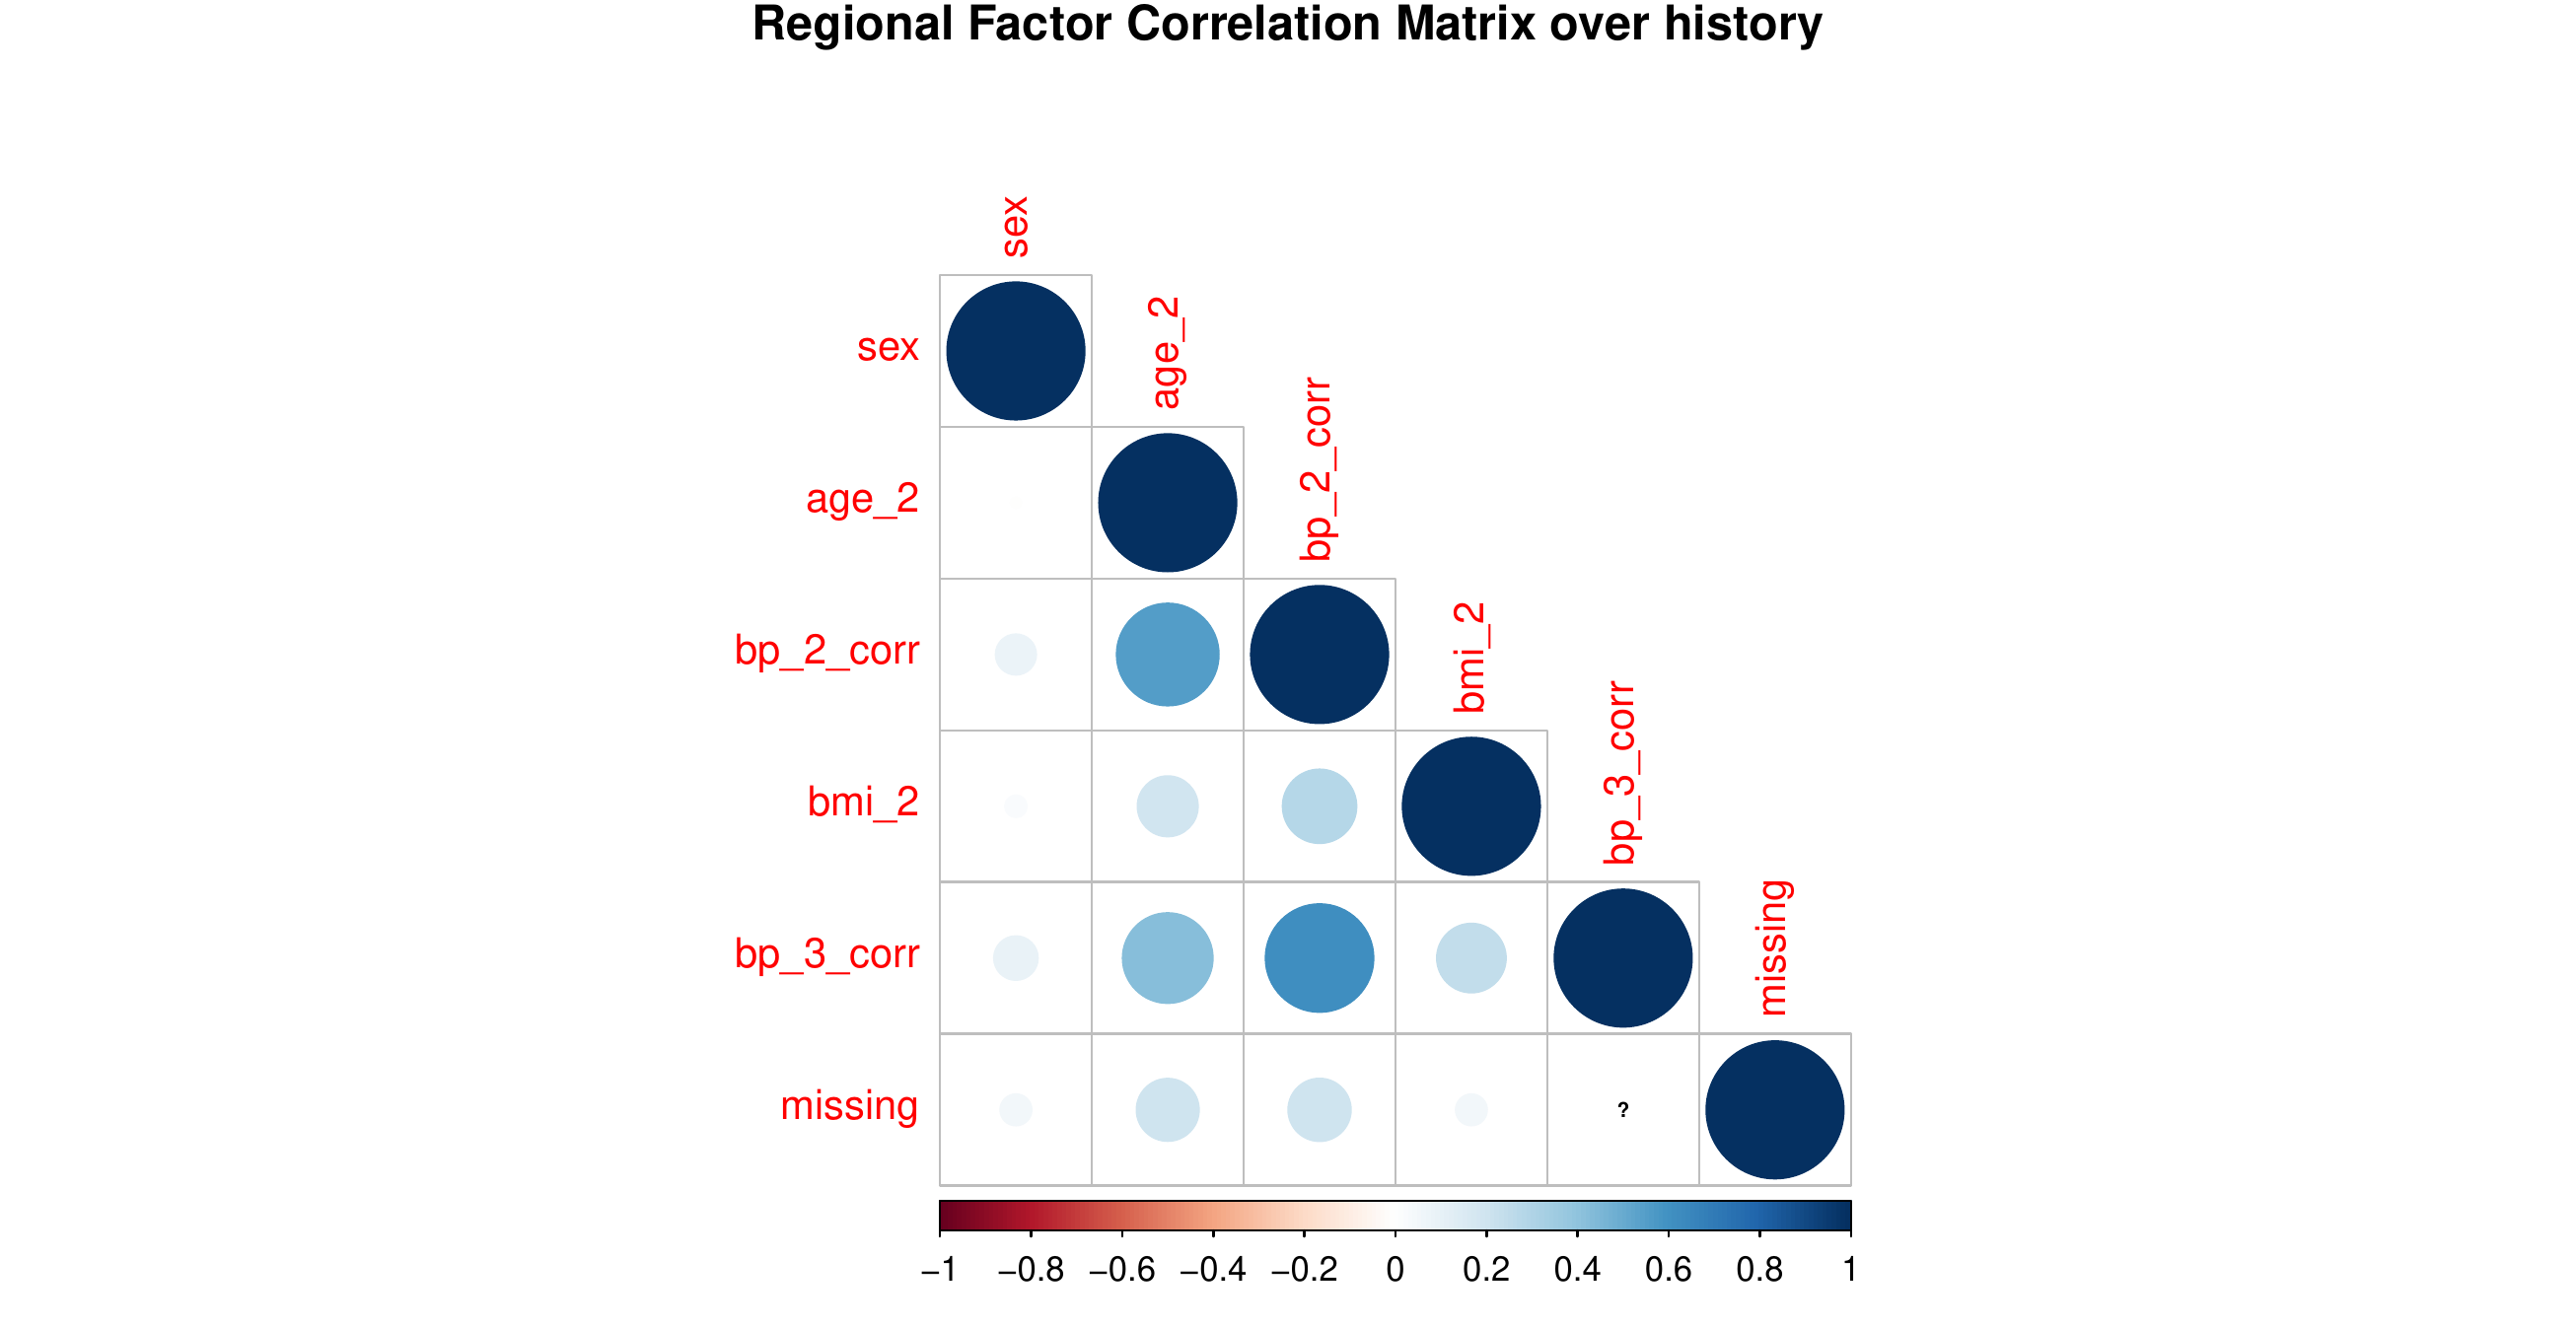}
        \caption{Correlation plot for simulated data.}
        \label{fig:corr_sim}
     \end{subfigure}
    \caption{}
    \label{fig:corr}
\end{figure}

For comparison concerning reproducibility purposes, we fitted our primary SPM \cref{eq:spm} and naive model \cref{eq:naive} to simulated data created as described in \cref{sec:reproducibility}. In the GitHub repository \cite{git_repo} two simulated datasets are available, one with $1000$ and one with $64385$ simulated participants. 
We see from \cref{fig:age_effect_sim_64385} and \cref{fig:parameter_est_sim_64385} that we obtain similar, although not identical, results for the model fits on the simulated dataset of the same size as the HUNT2 cohort as on the HUNT2 cohort. When we use the smaller simulated dataset with only $1000$ participants, we do not get the same results as for the real data. This can be seen in \cref{fig:age_effect_sim_1000} and \cref{fig:parameter_est_sim_1000}. We, therefore, note that while the smaller dataset can be used to verify the code, it can not be used to compare results. Further, we note that this indicates that a certain amount of data is needed for using the models presented in this work. 

\begin{figure}
    \centering
    \includegraphics[width=0.9\textwidth]{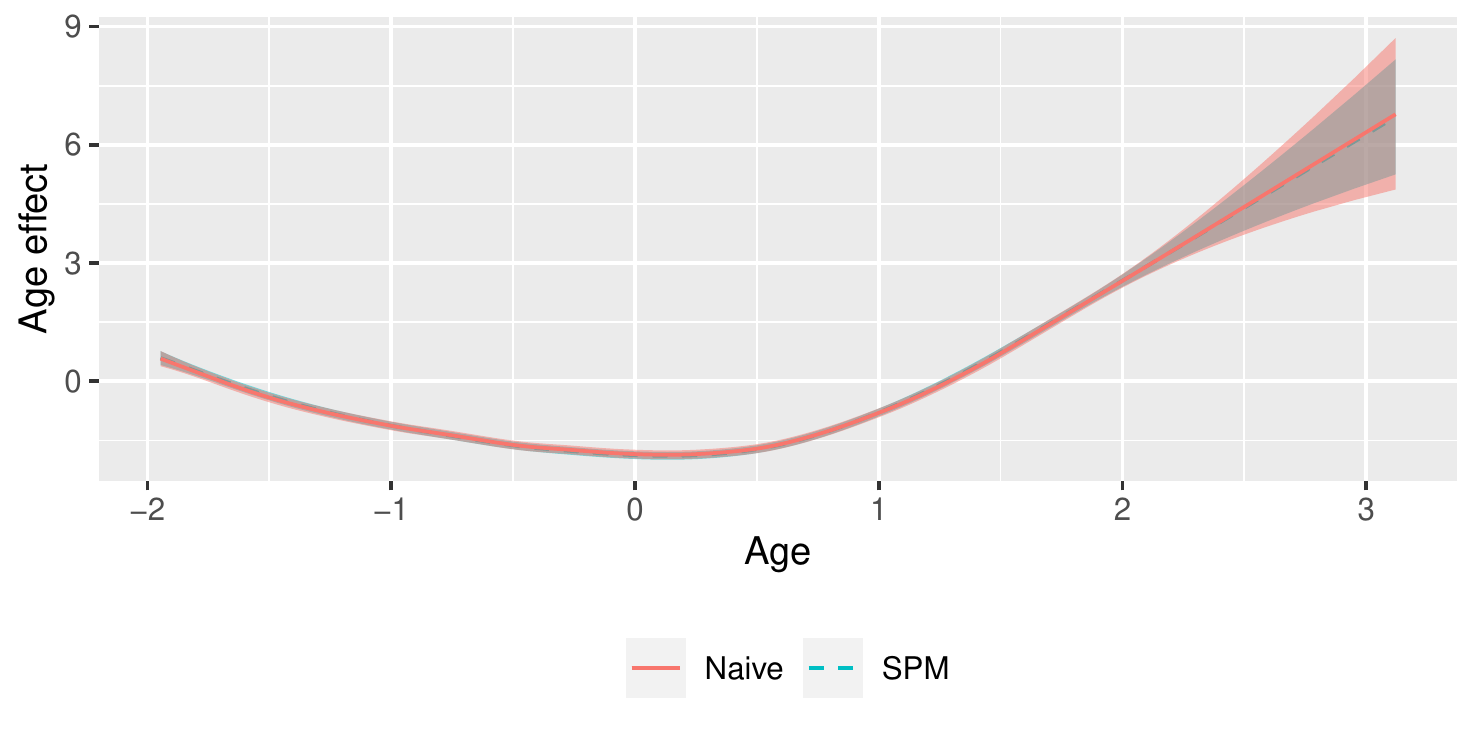}
    \caption{Age effect for the SPM and naive model fitted to simulated data mimicking the size ($64385$ participants) and structure of the HUNT2 cohort with $95\%$ credible bands.}
    \label{fig:age_effect_sim_64385}
\end{figure}

\begin{figure}
    \centering
    \includegraphics[width=0.9\textwidth]{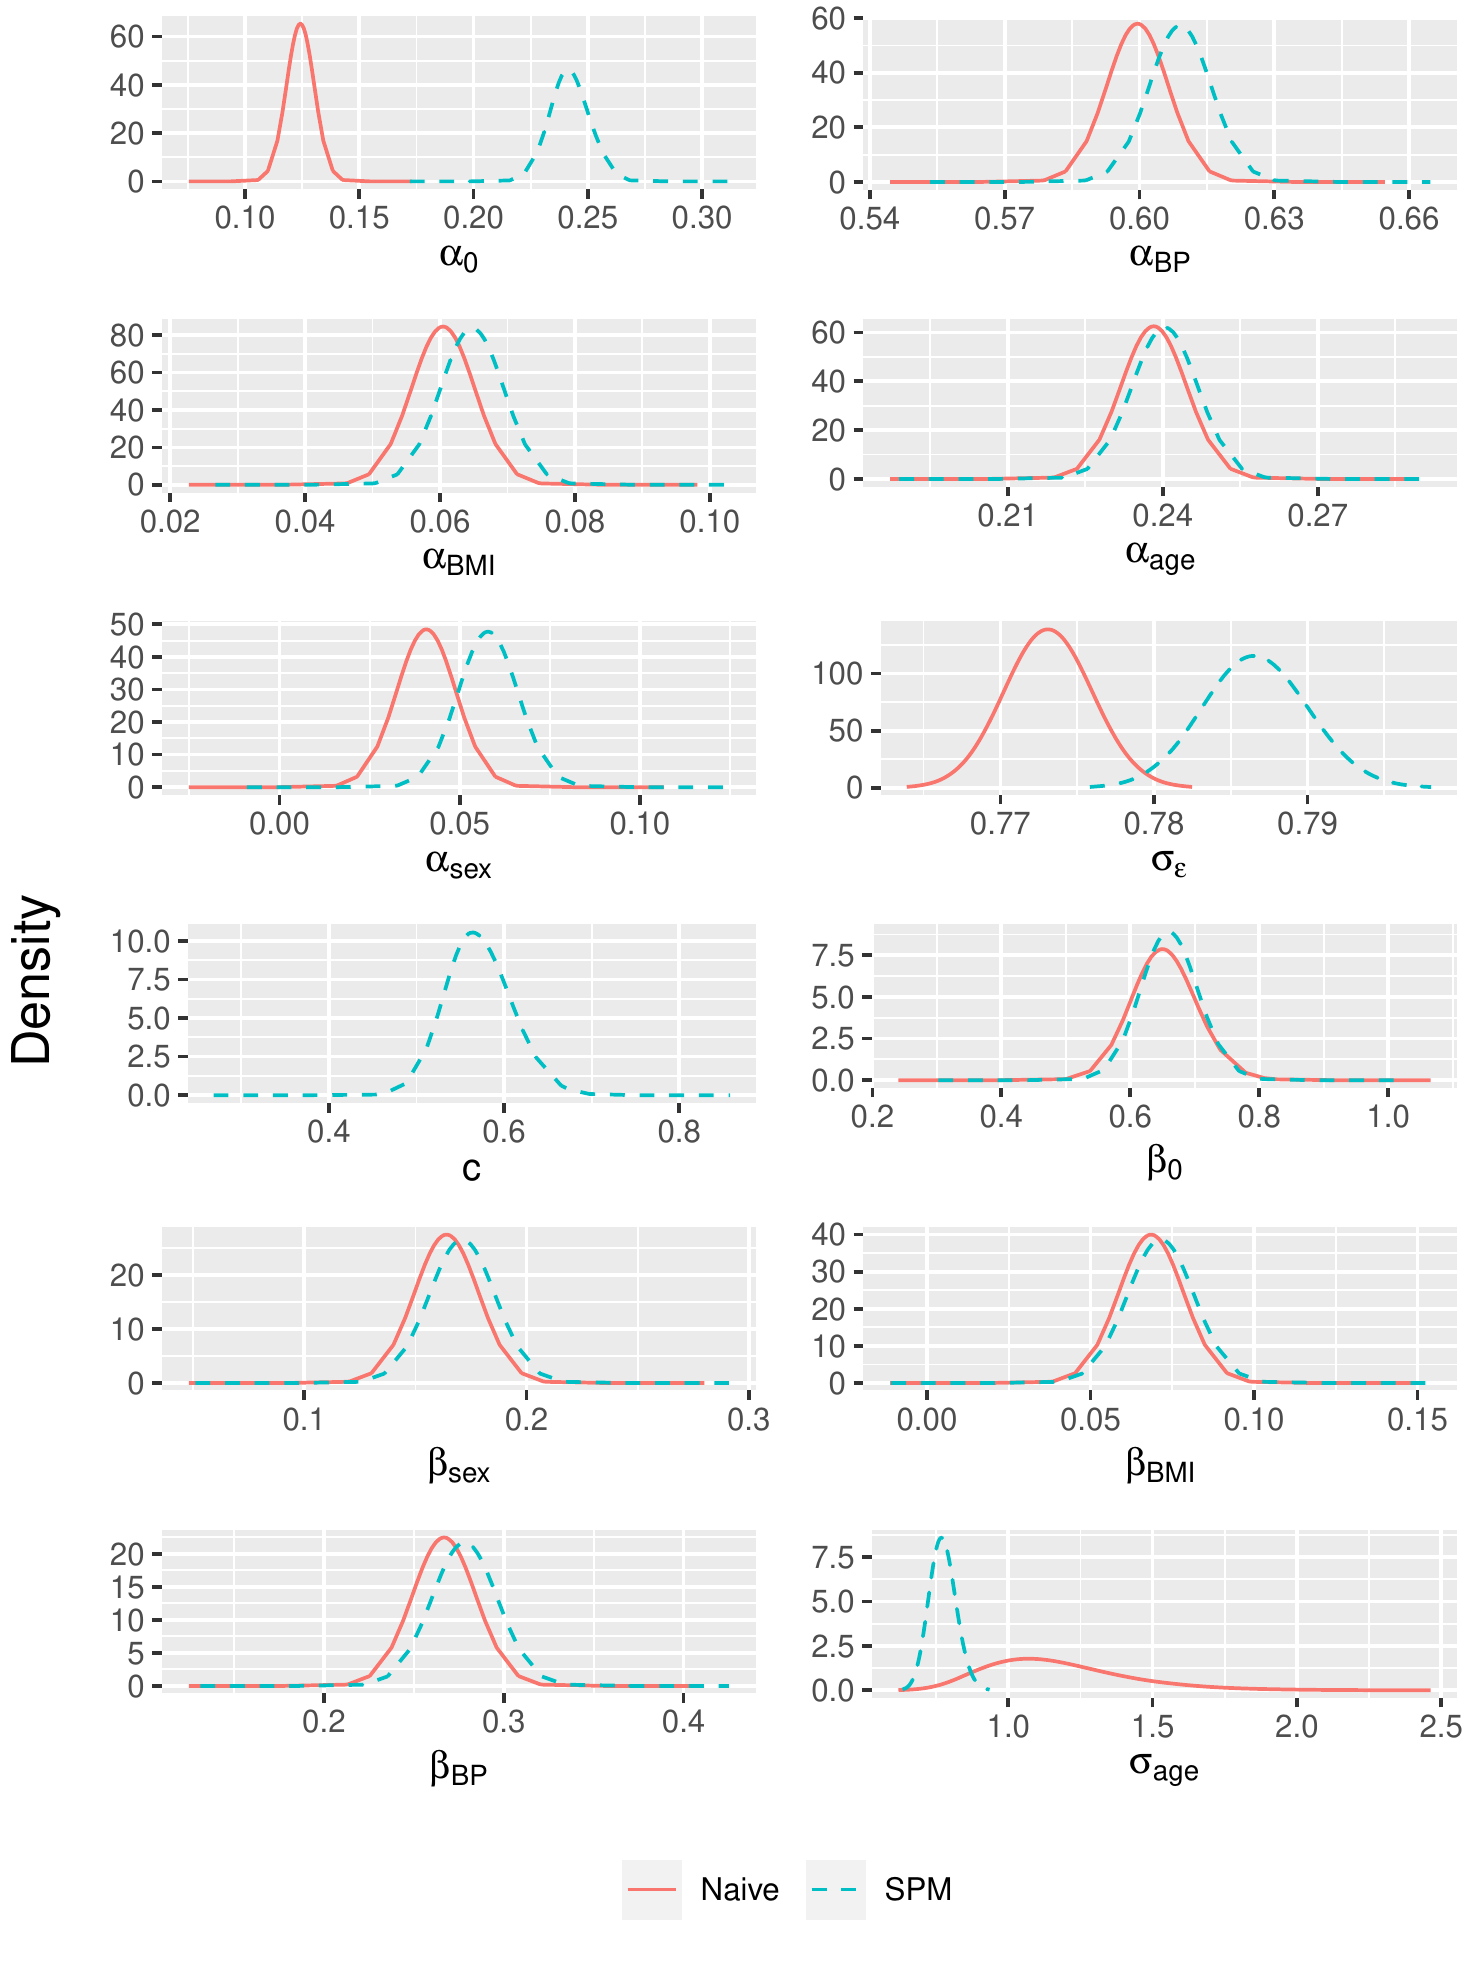}
    \caption{Posterior distribution of the latent field and hyperparameters for the SPM \cref{eq:spm} and naive model \cref{eq:naive} fitted to simulated data mimicking the size ($64385$ participants) and structure of the HUNT2 cohort.}
    \label{fig:parameter_est_sim_64385}
\end{figure}

\begin{figure}
    \centering
    \includegraphics[width=0.9\textwidth]{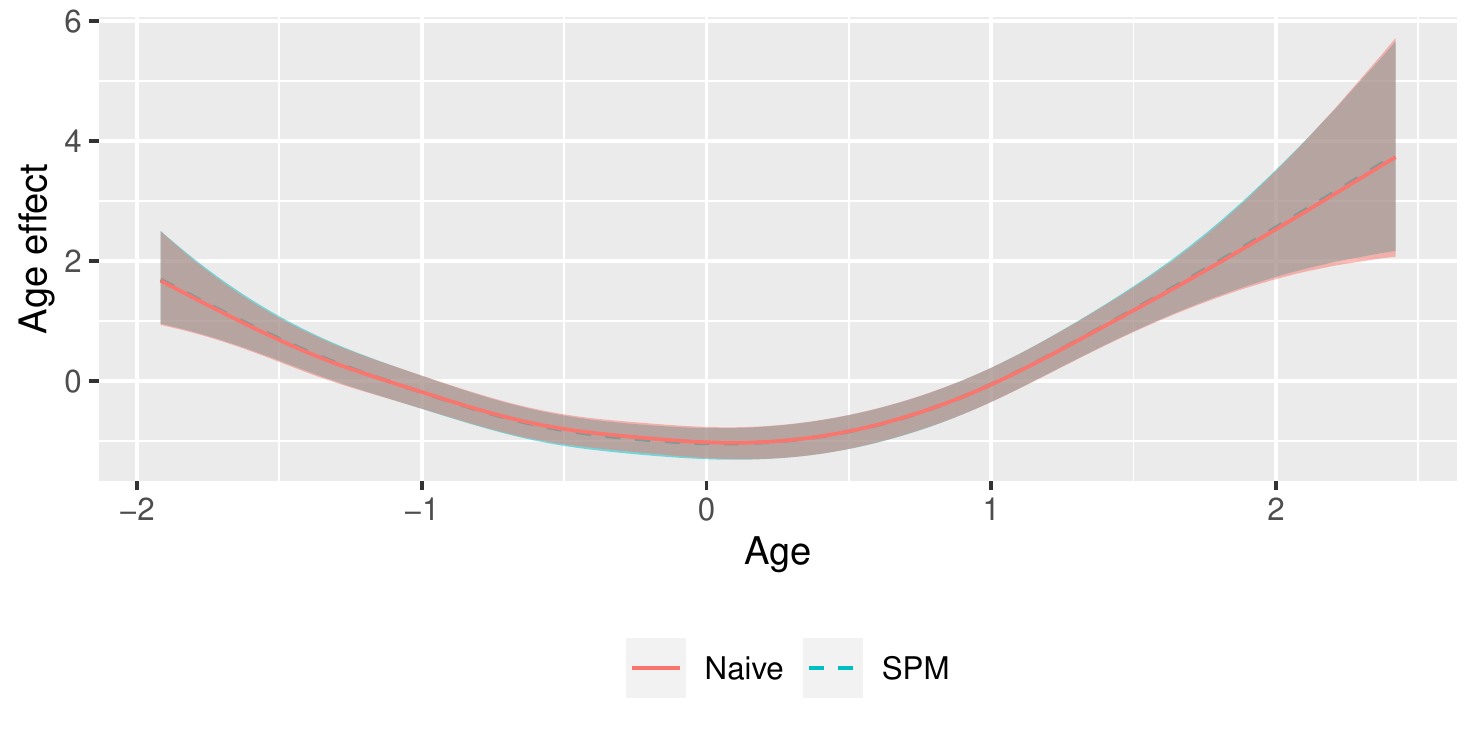}
    \caption{Age effect for the SPM and naive model fitted to a small simulated dataset ($1000$ participants) mimicking structure of the HUNT2 cohort with $95\%$ credible bands.}
    \label{fig:age_effect_sim_1000}
\end{figure}

\begin{figure}
    \centering
    \includegraphics[width=0.9\textwidth]{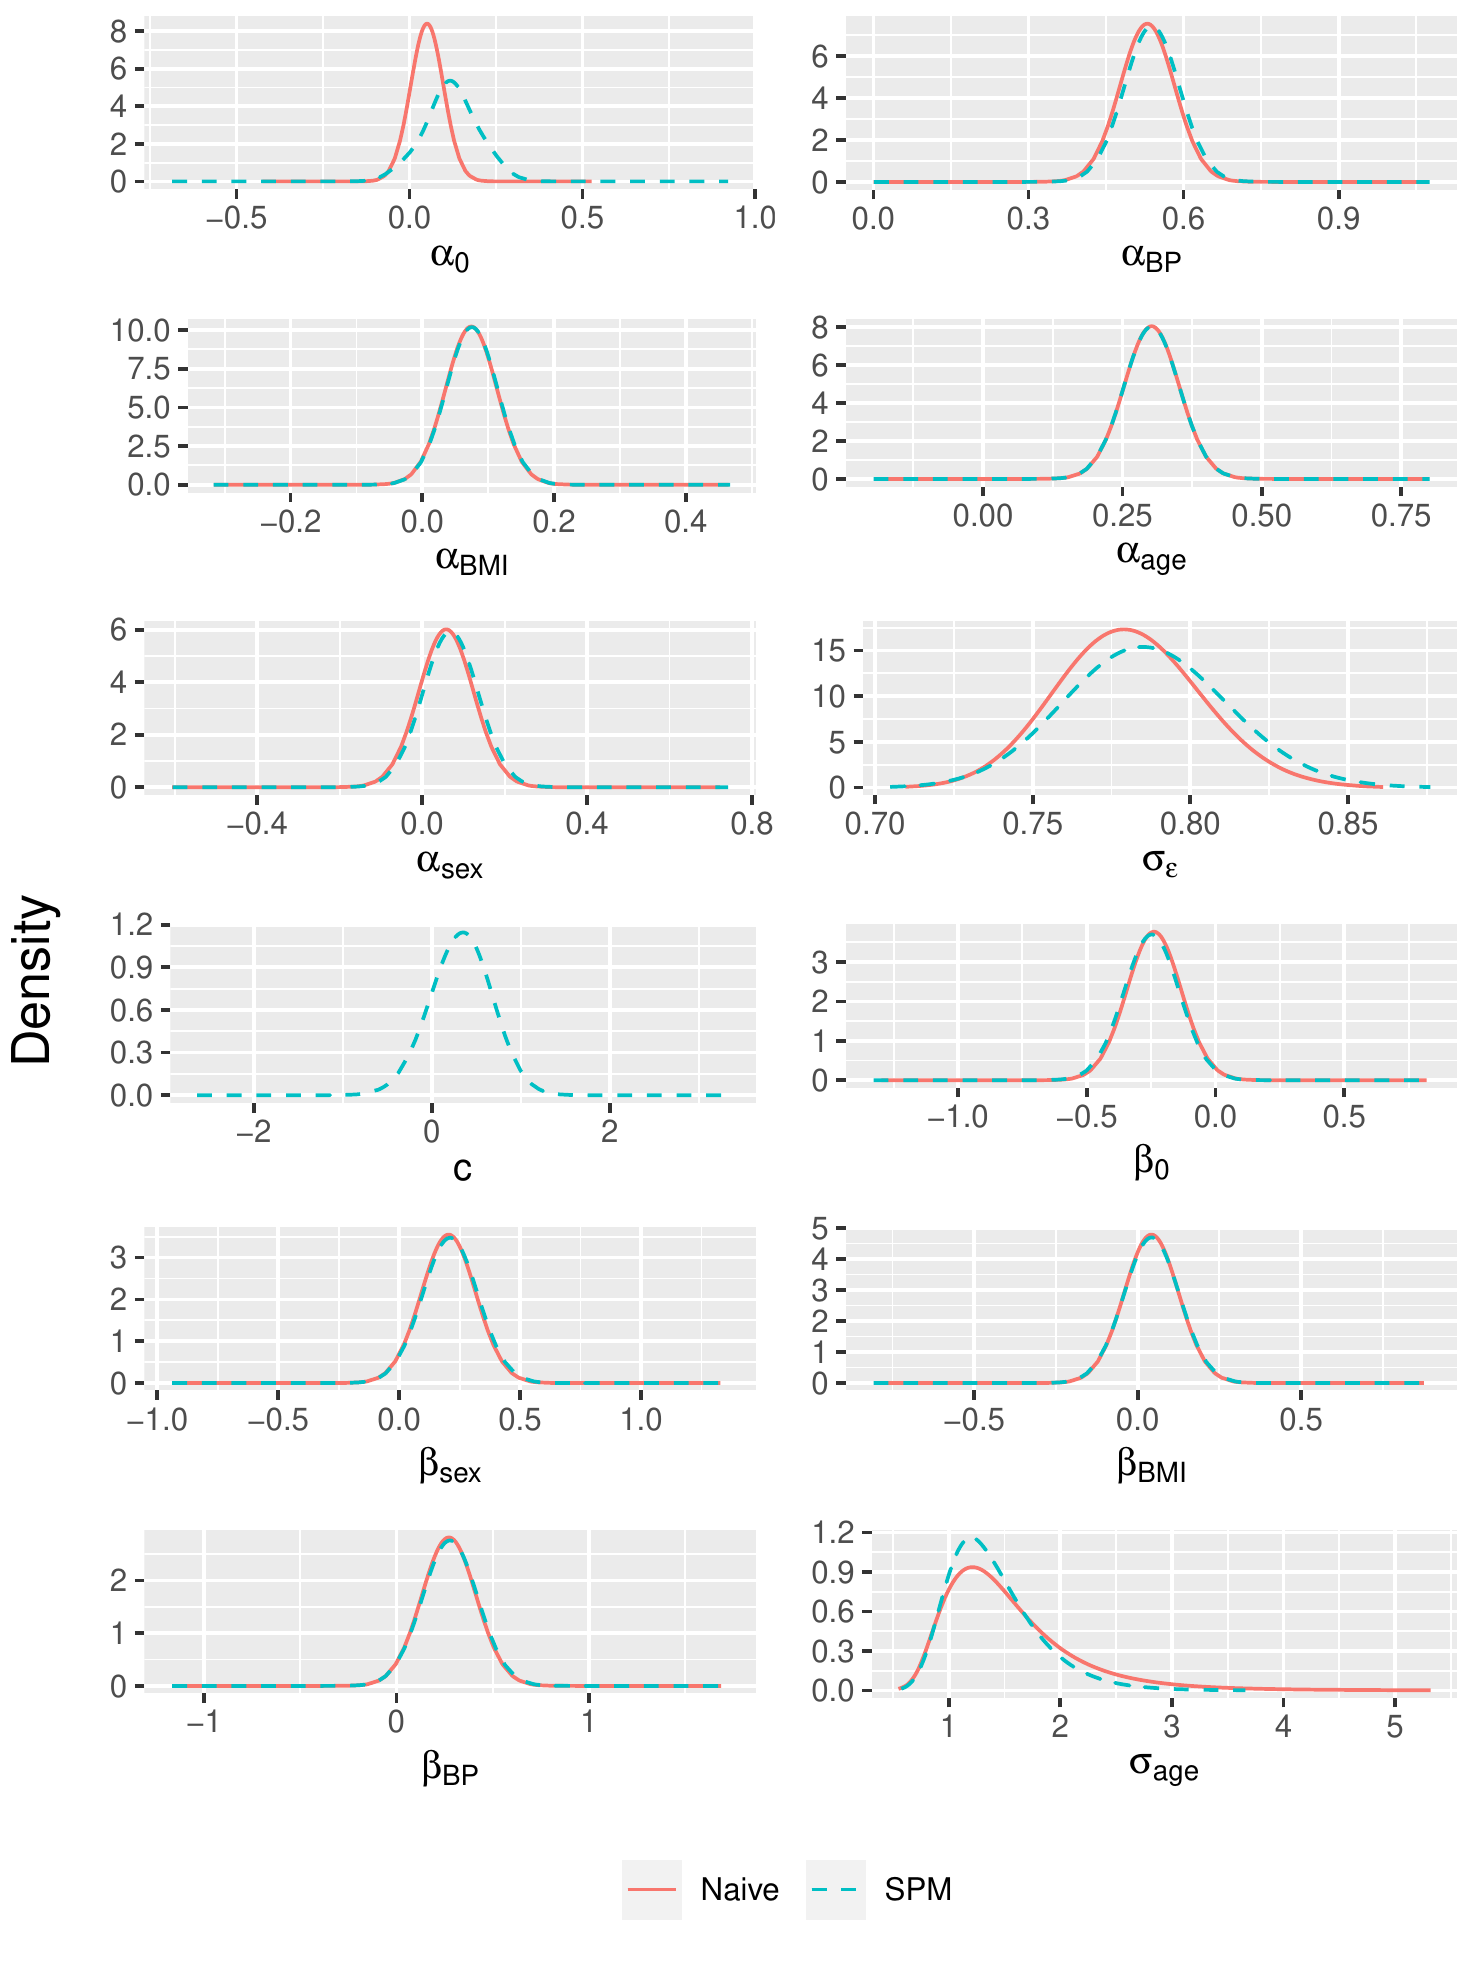}
    \caption{Posterior distribution of the latent field and hyperparameters for the SPM \cref{eq:spm} and naive model \cref{eq:naive} fitted to a small simulated dataset ($1000$ participants) mimicking the structure  of the HUNT2 cohort.}
    \label{fig:parameter_est_sim_1000}
\end{figure}

\begin{figure}
    \centering
    \includegraphics[width = \textwidth]{images/hist_comp_true_sim.pdf}
    \caption{Comparison of the distribution for $age, BMI, BP_2, BP_3$ from the HUNT2 cohort and simulated data.}
    \label{fig:sim_data_comp}
\end{figure}
