# Supplementary material for: A Shared Parameter Model for Systolic Blood Pressure Accounting for Data Missing Not at Random in the HUNT Study
Source: arXiv:2203.16602 source file (2022-03-30)
Supplement: Supplementary file 2 [file validation_model_predictions.tex]

\section{Simulation study on Model Predictions}
\label{sec:simulation_model_pred}
To test the validation scheme introduced in \cref{sec:validation_prediction} comparing the CRPS and Brier score of the model predictions for the SPM and naive model, we perform a simulation study with known data.
On actual data, we can only compute the CRPS score for the present participants. To explore how the CRPS score varies between the total population, the present, and the missing participants, we test the scheme on simulated data where we have $BP_F$ values for all $i$ participants.

\textbf{Setup:}

We use the posterior mean estimates obtained by the SPM introduced in \cref{sec:spm} (\Cref{tb:summary_param_est}) as the true values for the model parameters $
 \boldsymbol{\theta}_{true}$ = $(\hat{\alpha_0}$, $\hat{{\alpha}_{BP}}$, $\hat{{\alpha}_{age}}$, $\hat{{\alpha}_{BMI}}$, $\hat{{\alpha}_{sex}}$, $\hat{\beta_0}$, $\hat{{\beta}_{BP}}$, $\hat{{\beta}_{BMI}}$, $\hat{{\beta}_{sex}}$,  $\hat{c}$, $\hat{f(.)}$,  $\hat{{\sigma}_{\epsilon}}$).  
These are used to simulate values for the ${BP_F}_i$ and $m_i$, with explanatory variables from the HUNT2 cohort, identically as given in \cref{sec:sim_identifiability}. The simulated data is now MNAR and follows the SPM. 
Then we refit the SPM
and naive model
to this dataset and denote these model fits $SPM^*$ and $Naive*$, where $*$ denotes the new model fits.

The setup of the 100 simulations is as follows:

-- First we construct new values for $BP_F$ and $m$ similarly as in \cref{sec:sim_identifiability} but with explanatory variables from the HUNT3 cohort for all i participants.
This gives us a new dataset denoted $\text{data}_{new}$

-- Run the validation procedure as described in \cref{sec:validation_prediction} on $\text{data}_{new}$ with $SPM^*$ and $Naive*$ as model fits to obtain the mean CRPS score, $CRPS_l$, and the Brier score, $Brier_l$ for both the SPM and naive model.

We now have $100$ values of the mean CRPS score for the present and the missing participants, only the present, and only the missing participants in each simulation.

\textbf{Results and Discussion:}

Figure \cref{fig:diff_crps} displays the distribution of the difference between the mean CRPS for the SPM and the naive model. This difference is displayed for all simulations and grouped on missing status. We see that the SPM performs better for all participants and the dropouts, but the naive model performs better on present participants. This confirms our previous suspicion that even if the data is MNAR and the SPM fits the actual data better, the naive model is expected to obtain a better CRPS score when only tested on the present participants.

Figure \cref{fig:diff_brier} shows the distribution of the difference in Brier score for all participants, the dropouts, and the present participants. We see similar results here, although the Brier score for all participants, in this case, covers zero. However, for the dropout process, the original parameter estimates of the SPM and naive model (\cref{tb:summary_param_est}) were much more similar than for the $BP_F$ process. Naturally, these predictions will then be closer to one another.

\begin{figure}
    \centering
    \begin{subfigure}[b]{0.45\textwidth}
    \centering
    \includegraphics[width = \textwidth]{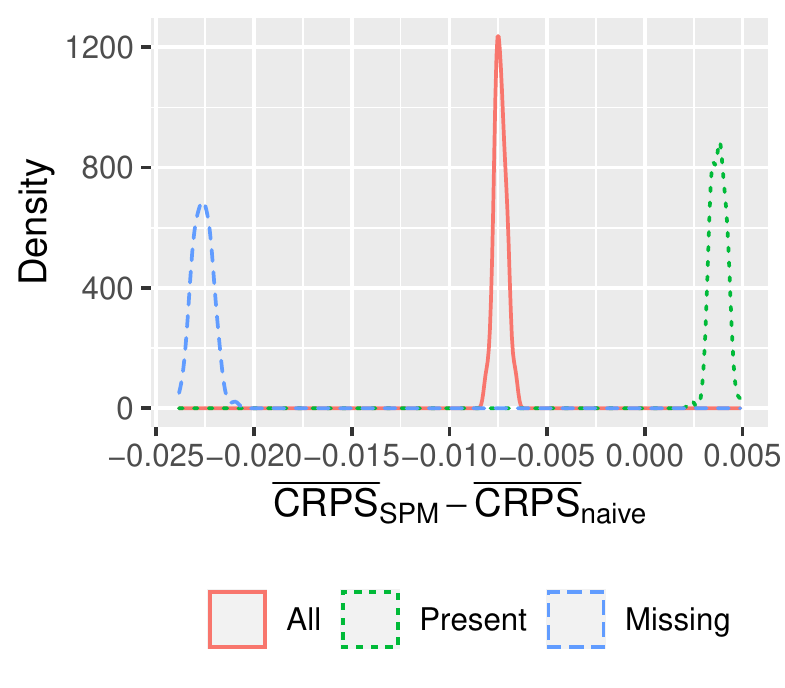}
    \caption{Difference in mean CRPS score for the SPM and naive model with 100 simulations} 
    \label{fig:diff_crps}
    \end{subfigure}
    ~
    \begin{subfigure}[b]{0.45\textwidth}
    \centering
    \includegraphics[width = \textwidth]{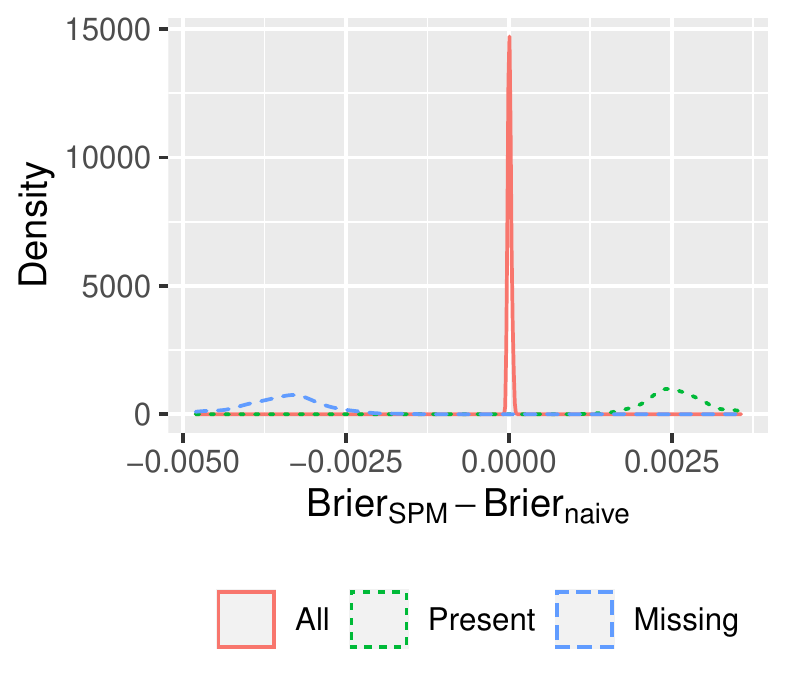}
    \caption{Difference in mean Brier score for the SPM and naive model with 100 simulations}
    \label{fig:diff_brier}
    \end{subfigure}
\end{figure}

To summarize, we find that the CRPS score for the $BP_F$ process can be better for the naive model than the SPM if we only consider the present participants. Otherwise, the CRPS of the SPM is the best if the data follows the SPM. The Brier score of the dropout process for the SPM is better for drop outs, very similar for the all participants (present and missing), and worse for the present participants than the naive model when the data follows the SPM.
